# Supplementary material for: Transmission Channel Analysis in Dynamic Models
Source: arXiv:2405.18987 source file (2026-10-23)
Supplement: Supplementary file 1 [file additional-figures.tex]

\section{Additional Figures}
\label{appendix:additional-figures}

\begin{figure}[H]
    \centering
    \begin{subfigure}{0.3\textwidth}
    \centering
    \begin{tikzpicture}[scale=0.6, transform shape]

        \node[circle, draw, line width=1pt, minimum size=1.22cm] (ffr) at (0, 6) {ffr};
        \node[circle, draw, line width=1pt, minimum size=1.22cm] (ygap) at (0, 4) {ygap};
        \node[circle, draw, line width=1pt, minimum size=1.22cm] (infl) at (0, 2) {infl};
        \node[circle, draw, line width=1pt, minimum size=1.22cm] (com) at (0, 0) {com};

        \draw[-latex, line width=1pt, mycolor1] (ffr) -- (ygap);
        \draw[-latex, line width=1pt, mycolor1] (ygap) -- (infl);
        \draw[-latex, line width=1pt, mycolor1] (infl) -- (com);
        \draw[-latex, line width=1pt, mycolor1] (ffr) edge [in=45, out=-45] (infl);
        \draw[-latex, line width=1pt, mycolor1] (ffr) edge [in=45, out=-40] (com);
        \draw[-latex, line width=1pt, mycolor1] (ygap) edge [in=60, out=-45] (com);

        \node[rectangle, draw=blue!50, fill=blue!20, line width=0.5pt, minimum size=0.3cm] (e) at (-2.0, 6) {$\varepsilon^i$};
        
        \draw[-latex, line width=1pt, mycolor1] (e) -- (ffr); 
        \draw[-latex, line width=1pt, black!10] (e) -- (ygap); 
        \draw[-latex, line width=1pt, black!10] (e) -- (infl); 
        \draw[-latex, line width=1pt, black!10] (e) -- (com); 
        
    \end{tikzpicture}
    \caption*{Contemporaneous}
    \end{subfigure}%
    \begin{subfigure}{0.3\textwidth}
    \centering
    \begin{tikzpicture}[scale=0.6, transform shape]

        \node[circle, draw, line width=1pt, minimum size=1.22cm, black!20] (ffr) at (0, 6) {\textcolor{black!20}{ffr}};
        \node[circle, draw, line width=1pt, minimum size=1.22cm] (ygap) at (0, 4) {ygap};
        \node[circle, draw, line width=1pt, minimum size=1.22cm] (infl) at (0, 2) {infl};
        \node[circle, draw, line width=1pt, minimum size=1.22cm] (com) at (0, 0) {com};

        \draw[-latex, line width=1pt, black!10] (ffr) -- (ygap);
        \draw[-latex, line width=1pt, mycolor2] (ygap) -- (infl);
        \draw[-latex, line width=1pt, mycolor2] (infl) -- (com);
        \draw[-latex, line width=1pt, black!10] (ffr) edge [in=45, out=-45] (infl);
        \draw[-latex, line width=1pt, black!10] (ffr) edge [in=45, out=-40] (com);
        \draw[-latex, line width=1pt, mycolor2] (ygap) edge [in=60, out=-45] (com);

        \node[rectangle, draw=blue!50, fill=blue!20, line width=0.5pt, minimum size=0.3cm] (e) at (-2.0, 6) {$\varepsilon^i$};
        
        \draw[-latex, line width=1pt, black!10] (e) -- (ffr); 
        \draw[-latex, line width=1pt, mycolor2] (e) -- (ygap); 
        \draw[-latex, line width=1pt, mycolor2] (e) -- (infl); 
        \draw[-latex, line width=1pt, mycolor2] (e) -- (com); 
        
    \end{tikzpicture}
    \caption*{Non-Contemporaneous}
    \end{subfigure}
    \caption{Illustration of the contemporaneous and non-contemporaneous transmission channels at horizon zero for the application in Section \ref{sec:sec5-mckay-wolf}. Greyed-out edges and nodes are not involved in the transmission channels. $ffr$ is the federal funds rate, $ygap$ is the output gap, $infl$ is price inflation, and $com$ is a commodity price index. The effect along the blue and yellow coloured edges are presented in Figure \ref{fig:instrument-comparison} at horizon zero by the blue and yellow bars respectively.}
    \label{fig:mckay-wolf-illustration}
\end{figure}

\begin{figure}[H]
    \centering
    \begin{subfigure}{0.3\textwidth}
    \centering
    \begin{tikzpicture}[scale=0.6, transform shape]

        \node[circle, draw, line width=1pt, minimum size=1.22cm] (news) at (0, 6) {news};
        \node[circle, draw, line width=1pt, minimum size=1.22cm, black!20] (gdef) at (0, 4) {\textcolor{black!20}{gdef}};
        \node[circle, draw, line width=1pt, minimum size=1.22cm] (gov) at (0, 2) {gov};
        \node[circle, draw, line width=1pt, minimum size=1.22cm] (gdp) at (0, 0) {gdp};

        \draw[-latex, line width=1pt, black!10] (news) -- (gdef);
        \draw[-latex, line width=1pt, black!10] (gdef) -- (gov);
        \draw[-latex, line width=1pt, mycolor1] (gov) -- (gdp);
        \draw[-latex, line width=1pt, mycolor1] (news) edge [in=45, out=-45] (gov);
        \draw[-latex, line width=1pt, mycolor1] (news) edge [in=45, out=-40] (gdp);
        \draw[-latex, line width=1pt, black!10] (gdef) edge [in=60, out=-45] (gdp);

        \node[rectangle, draw=blue!50, fill=blue!20, line width=0.5pt, minimum size=0.3cm] (e) at (-2.0, 6) {$\varepsilon^g$};
        
        \draw[-latex, line width=1pt, mycolor1] (e) -- (news); 
        \draw[-latex, line width=1pt, black!10] (e) -- (gdef); 
        \draw[-latex, line width=1pt, mycolor1] (e) -- (gov); 
        \draw[-latex, line width=1pt, mycolor1] (e) -- (gdp); 
        
    \end{tikzpicture}
    \caption*{Anticipation}
    \end{subfigure}%
    \begin{subfigure}{0.3\textwidth}
    \centering
    \begin{tikzpicture}[scale=0.6, transform shape]

        \node[circle, draw, line width=1pt, minimum size=1.22cm] (news) at (0, 6) {news};
        \node[circle, draw, line width=1pt, minimum size=1.22cm] (gdef) at (0, 4) {gdef};
        \node[circle, draw, line width=1pt, minimum size=1.22cm] (gov) at (0, 2) {gov};
        \node[circle, draw, line width=1pt, minimum size=1.22cm] (gdp) at (0, 0) {gdp};

        \draw[-latex, line width=1pt, mycolor2] (news) -- (gdef);
        \draw[-latex, line width=1pt, mycolor2] (gdef) -- (gov);
        \draw[-latex, line width=1pt, mycolor2] (gov) -- (gdp);
        \draw[-latex, line width=1pt, black!10] (news) edge [in=45, out=-45] (gov);
        \draw[-latex, line width=1pt, black!10] (news) edge [in=45, out=-40] (gdp);
        \draw[-latex, line width=1pt, mycolor2] (gdef) edge [in=60, out=-45] (gdp);

        \node[rectangle, draw=blue!50, fill=blue!20, line width=0.5pt, minimum size=0.3cm] (e) at (-2.0, 6) {$\varepsilon^g$};
        
        \draw[-latex, line width=1pt, mycolor2] (e) -- (news); 
        \draw[-latex, line width=1pt, mycolor2] (e) -- (gdef); 
        \draw[-latex, line width=1pt, black!10] (e) -- (gov); 
        \draw[-latex, line width=1pt, black!10] (e) -- (gdp); 
        
    \end{tikzpicture}
    \caption*{Implementation}
    \end{subfigure}%
    \caption{Illustration of the anticipation and implementation transmission channels at horizon zero for the application in Section \ref{sec:sec5-ramey}. Greyed-out edges and nodes are not involved in the transmission channels. $news$ represents the \citet{rameyDefenseNewsShocks2016} defense news series, $gdef$ is government defense spending, $gov$ is total government spending, and $gdp$ is real GDP. The effect along the blue and yellow coloured edges are presented in Figure \ref{fig:sec5-ramey} at horizon zero by the blue and yellow bars respectively.}
    \label{fig:ramey-illustration}
\end{figure}

\begin{figure}[H]
    \centering
    \begin{subfigure}{0.3\textwidth}
    \centering
    \begin{tikzpicture}[scale=0.6, transform shape]

        \node[circle, draw, line width=1pt, minimum size=1.1cm] (r) at (0, 6) {$r$};
        \node[circle, draw, line width=1pt, minimum size=1.1cm, black!20] (exp) at (0, 4) {\textcolor{black!20}{$\pi^e$}};
        \node[circle, draw, line width=1pt, minimum size=1.1cm, black!20] (y) at (0, 2) {\textcolor{black!20}{$x$}};
        \node[circle, draw, line width=1pt, minimum size=1.1cm] (p) at (0, 0) {$\pi$};

        \draw[-latex, line width=1pt, black!10] (r) -- (exp);
        \draw[-latex, line width=1pt, black!10] (exp) -- (y);
        \draw[-latex, line width=1pt, black!10] (y) -- (p);
        \draw[-latex, line width=1pt, black!10] (r) edge [in=45, out=-45] (y);
        \draw[-latex, line width=1pt, mycolor1] (r) edge [in=45, out=-40] (p);
        \draw[-latex, line width=1pt, black!10] (exp) edge [in=60, out=-45] (p);

        \node[rectangle, draw=blue!50, fill=blue!20, line width=0.5pt, minimum size=0.3cm] (e) at (-2.0, 6) {$\varepsilon^i$};
        
        \draw[-latex, line width=1pt, mycolor1] (e) -- (r); 
        \draw[-latex, line width=1pt, black!10] (e) -- (exp); 
        \draw[-latex, line width=1pt, black!10] (e) -- (y); 
        \draw[-latex, line width=1pt, mycolor1] (e) -- (p); 
        
    \end{tikzpicture}
    \caption*{Pure Interest Rate}
    \end{subfigure}%
    \hfill
    \begin{subfigure}{0.3\textwidth}
    \centering
    \begin{tikzpicture}[scale=0.6, transform shape]

        \node[circle, draw, line width=1pt, minimum size=1.1cm] (r) at (0, 6) {$r$};
        \node[circle, draw, line width=1pt, minimum size=1.1cm] (exp) at (0, 4) {$\pi^e$};
        \node[circle, draw, line width=1pt, minimum size=1.1cm, black!20] (y) at (0, 2) {\textcolor{black!20}{$x$}};
        \node[circle, draw, line width=1pt, minimum size=1.1cm] (p) at (0, 0) {$\pi$};

        \draw[-latex, line width=1pt, mycolor6] (r) -- (exp);
        \draw[-latex, line width=1pt, black!10] (exp) -- (y);
        \draw[-latex, line width=1pt, black!10] (y) -- (p);
        \draw[-latex, line width=1pt, black!10] (r) edge [in=45, out=-45] (y);
        \draw[-latex, line width=1pt, black!10] (r) edge [in=45, out=-40] (p);
        \draw[-latex, line width=1pt, mycolor6] (exp) edge [in=60, out=-45] (p);

        \node[rectangle, draw=blue!50, fill=blue!20, line width=0.5pt, minimum size=0.3cm] (e) at (-2.0, 6) {$\varepsilon^i$};
        
        \draw[-latex, line width=1pt, mycolor6] (e) -- (r); 
        \draw[-latex, line width=1pt, mycolor6] (e) -- (exp); 
        \draw[-latex, line width=1pt, black!10] (e) -- (y); 
        \draw[-latex, line width=1pt, black!10] (e) -- (p); 
        
    \end{tikzpicture}
    \caption*{Expectations}
    \end{subfigure}%
    \hfill
    \begin{subfigure}{0.3\textwidth}
    \centering
    \begin{tikzpicture}[scale=0.6, transform shape]

        \node[circle, draw, line width=1pt, minimum size=1.1cm] (r) at (0, 6) {$r$};
        \node[circle, draw, line width=1pt, minimum size=1.1cm] (exp) at (0, 4) {$\pi^e$};
        \node[circle, draw, line width=1pt, minimum size=1.1cm] (y) at (0, 2) {$x$};
        \node[circle, draw, line width=1pt, minimum size=1.1cm] (p) at (0, 0) {$\pi$};

        \draw[-latex, line width=1pt, mycolor2] (r) -- (exp);
        \draw[-latex, line width=1pt, mycolor2] (exp) -- (y);
        \draw[-latex, line width=1pt, mycolor2] (y) -- (p);
        \draw[-latex, line width=1pt, mycolor2] (r) edge [in=45, out=-45] (y);
        \draw[-latex, line width=1pt, black!10] (r) edge [in=45, out=-40] (p);
        \draw[-latex, line width=1pt, black!10] (exp) edge [in=60, out=-45] (p);

        \node[rectangle, draw=blue!50, fill=blue!20, line width=0.5pt, minimum size=0.3cm] (e) at (-2.0, 6) {$\varepsilon^i$};
        
        \draw[-latex, line width=1pt, mycolor2] (e) -- (r); 
        \draw[-latex, line width=1pt, mycolor2] (e) -- (exp); 
        \draw[-latex, line width=1pt, mycolor2] (e) -- (y); 
        \draw[-latex, line width=1pt, black!10] (e) -- (p); 
        
    \end{tikzpicture}
    \caption*{Output or Wage}
    \end{subfigure}
    \caption{Illustration of the pure-interest-rate, expectations, and output-wage transmission channels at horizon zero for the application in Section \ref{sec:sec5-dsge}. Greyed-out edges and nodes are not involved in the transmission channels. $r$ represents nominal interest rates, $\pi^e$ one period ahead rational expectations of inflation, $x=(y, c, i, w)$ summarises, for brevity, the vector of GDP ($y$), consumption ($c$), investment ($i$) and wages ($w$), and $\pi$ represents inflation. The effect along the blue, red, and yellow coloured edges are presented in Figure \ref{fig:sec5-dsge-decomposition} at horizon zero by the blue, red, and yellow bars respectively.}
    \label{fig:smets-wouters-illustratiokn}
\end{figure}

\begin{figure}[H]
    \centering
    \begin{subfigure}{0.3\textwidth}
    \centering
    \begin{tikzpicture}[scale=0.6, transform shape]

        \node[circle, draw, line width=1pt, minimum size=1.1cm] (r) at (0, 6) {r};
        \node[circle, draw, line width=1pt, minimum size=1.1cm, black!20] (exp) at (0, 4) {\textcolor{black!20}{x}};
        \node[circle, draw, line width=1pt, minimum size=1.1cm, black!20] (y) at (0, 2) {\textcolor{black!20}{$\pi^e$}};
        \node[circle, draw, line width=1pt, minimum size=1.1cm] (p) at (0, 0) {$\pi$};

        \draw[-latex, line width=1pt, black!10] (r) -- (exp);
        \draw[-latex, line width=1pt, black!10] (exp) -- (y);
        \draw[-latex, line width=1pt, black!10] (y) -- (p);
        \draw[-latex, line width=1pt, black!10] (r) edge [in=45, out=-45] (y);
        \draw[-latex, line width=1pt, mycolor1] (r) edge [in=45, out=-40] (p);
        \draw[-latex, line width=1pt, black!10] (exp) edge [in=60, out=-45] (p);

        \node[rectangle, draw=blue!50, fill=blue!20, line width=0.5pt, minimum size=0.3cm] (e) at (-2.0, 6) {$\varepsilon^i$};
        
        \draw[-latex, line width=1pt, mycolor1] (e) -- (r); 
        \draw[-latex, line width=1pt, black!10] (e) -- (exp); 
        \draw[-latex, line width=1pt, black!10] (e) -- (y); 
        \draw[-latex, line width=1pt, mycolor1] (e) -- (p); 
        
    \end{tikzpicture}
    \caption*{Pure Interest Rate}
    \end{subfigure}%
    \hfill
    \begin{subfigure}{0.3\textwidth}
    \centering
    \begin{tikzpicture}[scale=0.6, transform shape]

        \node[circle, draw, line width=1pt, minimum size=1.1cm] (r) at (0, 6) {r};
        \node[circle, draw, line width=1pt, minimum size=1.1cm] (exp) at (0, 4) {x};
        \node[circle, draw, line width=1pt, minimum size=1.1cm] (y) at (0, 2) {$\pi^e$};
        \node[circle, draw, line width=1pt, minimum size=1.1cm] (p) at (0, 0) {$\pi$};

        \draw[-latex, line width=1pt, mycolor6] (r) -- (exp);
        \draw[-latex, line width=1pt, mycolor6] (exp) -- (y);
        \draw[-latex, line width=1pt, mycolor6] (y) -- (p);
        \draw[-latex, line width=1pt, black!10] (exp) edge [in=60, out=-45] (p);
        \draw[-latex, line width=1pt, mycolor6] (r) edge [in=45, out=-45] (y);
        \draw[-latex, line width=1pt, black!10] (r) edge [in=45, out=-40] (p);

        \node[rectangle, draw=blue!50, fill=blue!20, line width=0.5pt, minimum size=0.3cm] (e) at (-2.0, 6) {$\varepsilon^i$};
        
        \draw[-latex, line width=1pt, mycolor6] (e) -- (r); 
        \draw[-latex, line width=1pt, mycolor6] (e) -- (exp); 
        \draw[-latex, line width=1pt, mycolor6] (e) -- (y); 
        \draw[-latex, line width=1pt, black!10] (e) -- (p); 
        
    \end{tikzpicture}
    \caption*{Expectations}
    \end{subfigure}%
    \hfill
    \begin{subfigure}{0.3\textwidth}
    \centering
    \begin{tikzpicture}[scale=0.6, transform shape]

        \node[circle, draw, line width=1pt, minimum size=1.1cm] (r) at (0, 6) {r};
        \node[circle, draw, line width=1pt, minimum size=1.1cm] (exp) at (0, 4) {x};
        \node[circle, draw, line width=1pt, minimum size=1.1cm, black!20] (e) at (0, 2) {\textcolor{black!20}{$\pi^e$}};
        \node[circle, draw, line width=1pt, minimum size=1.1cm] (p) at (0, 0) {$\pi$};

        \draw[-latex, line width=1pt, mycolor2] (r) -- (exp);
        \draw[-latex, line width=1pt, black!10] (exp) -- (y);
        \draw[-latex, line width=1pt, black!10] (y) -- (p);
        \draw[-latex, line width=1pt, black!10] (r) edge [in=45, out=-45] (y);
        \draw[-latex, line width=1pt, black!10] (r) edge [in=45, out=-40] (p);
        \draw[-latex, line width=1pt, mycolor2] (exp) edge [in=60, out=-45] (p);

        \node[rectangle, draw=blue!50, fill=blue!20, line width=0.5pt, minimum size=0.3cm] (e) at (-2.0, 6) {$\varepsilon^i$};
        
        \draw[-latex, line width=1pt, mycolor2] (e) -- (r); 
        \draw[-latex, line width=1pt, mycolor2] (e) -- (exp); 
        \draw[-latex, line width=1pt, black!10] (e) -- (y); 
        \draw[-latex, line width=1pt, black!10] (e) -- (p); 
        
    \end{tikzpicture}
    \caption*{Output or Wage}
    \end{subfigure}
    \caption{Illustration of the pure-interest-rate, expectations, and output-wage transmission channels at horizon zero for the application in Section \ref{sec:sec5-dsge}. Greyed-out edges and nodes are not involved in the transmission channels. $r$ represents nominal interest rates, $\pi^e$ one period ahead rational expectations of inflation, $x=(y, c, i, w)$ summarises, for brevity, the vector of GDP ($y$), consumption ($c$), investment ($i$) and wages ($w$), and $\pi$ represents inflation. The effect along the blue, red, and yellow coloured edges are presented in Figure \ref{fig:sec5-dsge-decomposition-alternative} at horizon zero by the blue, red, and yellow bars respectively.}
    \label{fig:smets-wouters-illustration-alternative}
\end{figure}
